# Supplementary material for: AssemState: Manual and Physical-State-Guided Reasoning for Zero-shot Furniture Assembly
Source: arXiv:2610.08446 source file (2026-11-09)
Supplement: Supplementary file 1 [file appendix_only_preview.tex]

\documentclass[letterpaper]{article}
\usepackage[dblblindworkshop]{neurips_2026}
\workshoptitle{Physical World AI: Geometry, Characteristics, and Multimodal Sensing}

\usepackage[utf8]{inputenc}
\usepackage[T1]{fontenc}
\usepackage{hyperref}
\usepackage{url}
\usepackage{graphicx}
\usepackage{booktabs}
\usepackage{amsfonts}
\usepackage{nicefrac}
\usepackage{microtype}
\usepackage{xcolor}
\usepackage[most]{tcolorbox}

% Appendix palette matched to Fig. 2 / the main pipeline figure.
% Stage 1: blue; Stage 2 / pose loop: green; Stage 3: coral; feedback: orange.
\definecolor{StageOneBorder}{HTML}{2E54A1}
\definecolor{StageOneTitle}{HTML}{B1D2E1}
\definecolor{StageOneBack}{HTML}{F7F9FD}
\definecolor{StageTwoBorder}{HTML}{588E31}
\definecolor{StageTwoTitle}{HTML}{ACD78E}
\definecolor{StageTwoBack}{HTML}{F7FBF4}
\definecolor{StageThreeBorder}{HTML}{C00000}
\definecolor{StageThreeTitle}{HTML}{EF949E}
\definecolor{StageThreeBack}{HTML}{FFF8F3}
\definecolor{FeedbackBorder}{HTML}{EE822F}
\definecolor{FeedbackTitle}{HTML}{F6D3AE}
\definecolor{FeedbackBack}{HTML}{FFF9F1}
\definecolor{NeutralBorder}{HTML}{2E54A1}
\definecolor{NeutralTitle}{HTML}{DAE3F5}
\definecolor{NeutralBack}{HTML}{FAFBFE}

\tcbset{
  appendixbox/.style={
    enhanced,
    breakable,
    boxrule=0.8pt,
    arc=1.0mm,
    outer arc=1.0mm,
    left=1.8mm,
    right=1.8mm,
    top=0.9mm,
    bottom=1.2mm,
    before skip=5pt,
    after skip=7pt,
    fonttitle=\bfseries\small,
    coltitle=black,
    title filled,
    colbacktitle=white,
    toptitle=0.8mm,
    bottomtitle=0.8mm,
    lefttitle=1.2mm,
    righttitle=1.2mm
  }
}

\tcbset{
  StageOne/.style={colframe=StageOneBorder,colback=StageOneBack,colbacktitle=StageOneTitle},
  StageTwo/.style={colframe=StageTwoBorder,colback=StageTwoBack,colbacktitle=StageTwoTitle},
  StageThree/.style={colframe=StageThreeBorder,colback=StageThreeBack,colbacktitle=StageThreeTitle},
  PoseStage/.style={colframe=StageTwoBorder,colback=StageTwoBack,colbacktitle=StageTwoTitle},
  FeedbackStage/.style={colframe=FeedbackBorder,colback=FeedbackBack,colbacktitle=FeedbackTitle},
  NeutralStage/.style={colframe=NeutralBorder,colback=NeutralBack,colbacktitle=NeutralTitle}
}

\newcommand{\PromptFileBox}[3]{%
\begin{tcolorbox}[appendixbox,#1,title={#2}]
\VerbatimInput[fontsize=\scriptsize,breaklines=true,breakanywhere=true]{#3}
\end{tcolorbox}%
}

\newcommand{\OutputFileBox}[2]{%
\begin{tcolorbox}[appendixbox,StageTwo,title={#1}]
\VerbatimInput[fontsize=\small,breaklines=true,breakanywhere=true]{#2}
\end{tcolorbox}%
}

\newcommand{\CodeFileBox}[2]{%
\begin{tcolorbox}[appendixbox,NeutralStage,title={#1}]
\VerbatimInput[fontsize=\small,breaklines=true,breakanywhere=true]{#2}
\end{tcolorbox}%
}

\newcommand{\ProtocolBox}[3]{%
\begin{tcolorbox}[appendixbox,#1,title={#2}]
#3
\end{tcolorbox}%
}

\usepackage{amsmath}
\usepackage{amssymb}
\usepackage{booktabs}
\usepackage{multirow}
\usepackage{array}
\usepackage{tabularx}
\usepackage{ragged2e}
\usepackage{fvextra}
\usepackage{float}

\graphicspath{{latex/}}

\newcolumntype{L}[1]{>{\RaggedRight\arraybackslash}p{#1}}
\newcolumntype{Y}{>{\RaggedRight\arraybackslash}X}

\setcounter{secnumdepth}{0}

\title{FurniReason: Zero-Shot Vision-Language Reasoning for Manual-Guided Furniture Assembly}
\author{Paper ID: 38061}
\author{ontent Areas:CV:Vision for Robotics, Embodied \& Autonomous Driving}

\begin{document}
\input{latex/sec/appendix}
\end{document}
